# Supplementary material for: Stochastic Shortest Path with Energy Constraints in POMDPs
Source: arXiv:1602.07565 source file (2016-05-11)
Supplement: Supplementary file 1 [file appendix.tex]

%!TEX root = main.tex

\section{Details of Section~\ref{sec:prelim}}
\label{app:sec:prelim}
\subsection{Construction for Remark~\ref{rem:det-obs}}

% \begin{remark}[Deterministic observation function]
We remark that deterministic observation functions of type $\obsfunc : S \rightarrow \obs$ are sufficient in POMDPs.
Given a POMDP $\pomdp=(S,\acts,\tran,\obs,\obsfunc,\initdist_0)$, the most general type
of the observation function $\obsfunc$ considered in the literature is of type 
$\obsfunc: S \times \acts \rightarrow \distr(\obs)$, i.e., the state and the action 
gives a probability distribution over the set of observations $\obs$. 
We show how to transform the POMDP $\pomdp$ into one where the observation function 
is deterministic and defined on states, i.e., of type $\obsfunc' : S \rightarrow \obs$. 
We construct an equivalent polynomially larger POMDP $\pomdp'=(S',\acts,\tran',\obs,\obsfunc',\initdist_0')$
as follows: 
(i)~the new state space is $S' = S \times \obs$; 
(ii)~the transition function $\tran'$ given a state $(s,z) \in S'$ and an action $a$ 
is as follows $\tran'((s,z),a)(s',z') = \tran(s,a)(s') \cdot \obsfunc(s',a)(z')$; and
(iii) the deterministic observation function for a state $(s,z) \in S'$ is defined as $\obsfunc'((s,z)) 
= z$.
Informally, the probabilistic aspect of the observation function is captured in the 
transition function, and by enlarging the state space with the product with the observations,
we obtain an observation function only on states.
Thus in the sequel without loss of generality we will always consider observation function of type $\obsfunc' : S \rightarrow \obs$ 
which greatly simplifies the notation.
% \end{remark}

\section{Details of Section~\ref{sec:prelim}}
\label{app:sec:exp}

\subsection{Hallway problems.}
We consider two versions of the Hallway problems introduced in~\cite{LCK95} and used later in~\cite{S04,SS04,BG09}.
An example of a Hallway instance is depicted in Figure~\ref{fig:app_hallway2}. 
The basic idea behind the Hallway problems, is that there is an agent 
wandering around an office building. 
It is assumed that the locations have been discretized so there are a finite number of 
locations where the agent could be.  There are four different states as depicted in Figure~\ref{fig:app_hallway2}:
(i)~the agent starts uniformly at random in one of the \texttt{+} labeled states; (ii) the \texttt{R} labeled states
are the \emph{reload} states where the agents energy level is restored; (iii) the \texttt{X} labeled states are the \emph{trap}
states, once an agent visits a trap state it can never leave; and (iv) the \texttt{G} labeled states are the \emph{goal} states the agent
is trying to reach. In these problems the location in the building and the agent's current orientation comprise the states.
The agent has a small finite set of actions it can take. 
Every move of the agent has a uniform cost of $1$ and also decreases the energy level by $1$

\begin{figure}[h!]
\centering
\resizebox{5cm}{!}{
\input{hallway2}
}
\caption{An example of a Hallway instance}
\label{fig:app_hallway2}
\end{figure}

\subsection{RockSample problems.}
We consider a modification of the RockSample problem introduced in~\cite{SS04} and used later in~\cite{BG09}. It is a scalable problem that models
 rover science exploration. The rover is equipped with a limited amount of fuel and can
 increase the amount of fuel by sampling rocks in the immediate area.
   The positions of the rover and the rocks are known, but only some of the rocks can increase the energy level; we will call these 
   rocks good. The type of the rock is not known to the rover, until the rock is sampled.
Once a good rock is used to increase the amount of fuel, it becomes a bad rock and can't be used anymore to increase the energy level

An instance of the RockSample problem is parametrized with two parameters $[n,k]$: map size $n \times n$ and $k$ rocks 
is described as RockSample[n,k]. The POMDP model of RockSample[n,k] is as follows:

The instance RS[4,2] (resp. RS[4,3]) is depicted on Figure~\ref{fig:rs_small} (resp. Figure~\ref{fig:rs_large}), the arrow indicates 
the initial position of the rover and the filled rectangles denote the fixed positions of the rocks.
Every move of the rover has a uniform cost of $1$ and also decreases the energy level by $1$, with the exception of the sampling action
that decreases the energy level by $2$.

\begin{figure}[ht]
\centering
  \begin{minipage}[b]{0.40\linewidth} % A minipage that covers half the page
    \centering
    \resizebox{\linewidth}{!}{
    \begin{tikzpicture}[]
        \draw (0, 0) grid (4, 4);
        
        \fill [pattern=north west lines, pattern color=blue] (1,2) rectangle (2,3);
        \fill [pattern=north west lines, pattern color=blue] (3,0) rectangle (4,1);
        \draw[->]
        (-0.5,2.5) edge[ultra thick] node[above] {} (0.5,2.5);
        
        \draw [ultra thick] (0,0) rectangle (4,4);
    \end{tikzpicture}
    }
   \caption{RS[4,2]}
   \label{fig:rs_small}
  \end{minipage}
  \hspace{1.5cm}
  \begin{minipage}[b]{0.40\linewidth}
    \centering
 \centering
    \resizebox{\linewidth}{!}{
    \begin{tikzpicture}[]
        \draw (0, 0) grid (4, 4);
        \fill [pattern=north west lines, pattern color=blue] (1,3) rectangle (2,4);
        \fill [pattern=north west lines, pattern color=blue] (0,0) rectangle (1,1);
        \fill [pattern=north west lines, pattern color=blue] (2,1) rectangle (3,2);
        \draw[->]
        (-0.5,2.5) edge[ultra thick] node[above] {} (0.5,2.5);

        \draw [ultra thick] (0,0) rectangle (4,4);
    \end{tikzpicture}
    }
   \caption{RS[4,3]}
   \label{fig:rs_large}
  \end{minipage}
\end{figure}
